# Supplementary material for: Magnetic anisotropy in single-crystalline antiferromagnetic Mn$_2$Au
Source: arXiv:2404.15525 source file (2024-08-08)
Supplement: Supplementary file 1 [file Mn2Au_Supplement.pdf]

# Magnetic anisotropy in single-crystalline antiferromagnetic $Mn_2Au$

## Supporting Information

Mebatsion S. Gebre, Rebecca K. Banner, Kisung Kang, Kejian Qu, Huibo Cao, André Schleife, Daniel P. Shoemaker

# 1 Distribution of phases

The scanning electron microscopy (SEM) energy-dispersive X-ray spectroscopy (EDS) map in Figure S1 shows large clean areas of $Mn_2Au$ composition on single crystals grown from flux. However, some bismuth, in green, remains coating parts of the sample, especially in cracks and step-like features.

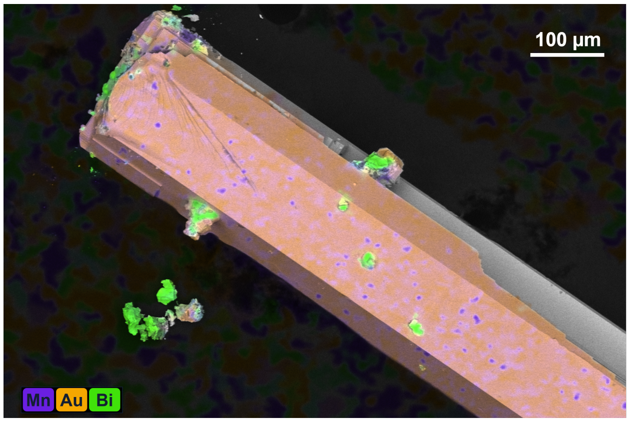


Figure S1: SEM-EDS of a rectangular $Mn_2Au$ crystal (orange/purple) with remnant Bi flux (green).

# 2 Further sample characterization

Magnetization isotherms and temperature sweeps were used to characterize the magnetic response of samples over a large span of temperatures between 10 K and 700 K. The characterizations help isolate the intrinsic responses of $Mn_2Au$ from the ferromagnetic MnBi impurity. Figure S5 shows magnetization isotherms of a $Mn_2Au$ crystal at 300 K (black) and at 700 K (red). The room temperature scan is overwhelmed by the ferromagnetic contribution from the MnBi impurity as evidenced by the large magnitude of magnetization $M$, the S-shaped saturation behavior, and a hysteresis extending to applied field $H = 2$ T. The

amount of MnBi in the sample is calculated to be ∼2 mol % by comparing the magnitude of saturation magnetization with a measurement of MnBi powder.

To confirm that the source of this ferromagnetic (FM) behavior is the MnBi impurity, the magnetization was traced between 300 K and 700 K as shown in Figure S4. Here, the black curve is data taken while heating the as-synthesized $Mn_2Au$ crystal. The blue curve shows magnetization data from the same run while cooling from 700 K. The abrupt loss of magnetic moment upon heating near 630 K corresponds to the expected phase change and magnetic disordering of MnBi at the same temperature [1]. The isotherm taken at 700 K after this first heating step, shown in red in Figure S5, traces a linear relationship for $M$ versus $H$ for the entire range of applied field between -7 T and 7 T, with a susceptibility value of $4.5 \pm 0.4^{-4}$. This linear relation is characteristic of antiferromagnetic and paramagnetic materials. The susceptibility of this curve at 700 K can be attributed to that of antiferromagnetic $Mn_2Au$, as it is in the order of magnitude expected [2]. While a paramagnetic contribution from MnBi is possible at this high temperature, it is negligible due to its relative amount. The disappearance of FM behavior above the Curie temperature of the MnBi impurity supports the hypothesis that the FM saturation (S-shape) observed at room temperature is not an intrinsic property of the $Mn_2Au$ sample itself, but rather of the MnBi impurity.

The FM signal from MnBi is partially lost after heating owing to decomposition of MnBi into the high-temperature orthorhombic polymorph that has a lower ordering temperature [3] as well as some minor oxidation of the surface to form $Mn_3O_4$. The magnetization measured on cooling from 700 K, blue curve in Figure S4, has a much lower magnitude than the heating curve. Further, it has sharp ordering-like transitions at 591 K and 512 K. The transition at 591 K is 22 K lower than the lowest temperature at which MnBi-high temperature phase (HTP) forms. The transition at 512 K is 23 K lower than the eutectic formation of MnBi-low temperature phase (LTP) from Mn-containing liquid Bi at 535 K according to the Mn-Bi phase diagram [4]. This slight undercooling can be expected due to the relatively fast cooling rate of 3 K/min. The magnetic ordering of the high-temperature-phase MnBi into its ferromagnetic state at 440 K [5] does not appear in this data. Thus the FM contribution to the magnetization significantly declines after being heated to 700 K and cooled quickly, so this heat treatment can be used as a way to suppress the FM signal and observe the linear $M$ versus $H$ regime within accessible applied fields.

In the main body of the paper, clean parts of the sample were cleaved to physically remove FM contributions from MnBi-containing flux. Cleaving the sample is advantageous because the sample stoichiometry and phase are unchanged, however it also gives significantly smaller samples with small moment magnitudes. Additional magnetic measurement results are presented here where alternative ways to suppress/avoid large impurity FM contributions at room temperature are used. In the first approach inspired by high-temperature magnetization measurements, a sample was heated to 700 K in vacuum to avoid oxidation and quenched quickly to avoid reformation of the LTP-MnBi phase (Fig. S6). In the second approach, the $Mn_2Au$ crystals were etched with a 1:2 HCl and $HNO_3$ solution for 2 minutes to remove the bismuth flux (Fig. S7). Leftover flux on the exposed flat surfaces of the crystal was easily removed with this second method, but some Bi flux lining the crevices and step-like facets of the crystals was not fully etched. Because Mn is much more susceptible to acid etching than Au [6, 7], the top layer of the etched crystals is depleted of Mn and appears golden. We assume that the diamagnetic contribution of the Au layer on these crystals has

negligible effect on the magnetization characterizations.

Magnetization versus field curves at and below 300 K were then taken on the heat treated and acid cleaned samples along different crystal directions to probe anisotropy. In both cases, heating to above the Curie temperature of MnBi or etching significantly reduces the FM signal, which allows access to the AFM-dominated linear behavior in M vs H curves above 3 T. Susceptibility $\chi$ is calculated using the slope of the linear section of the data for applied fields above 3 T. Figure S6 shows isotherms taken at 10 K and at 300 K for field applied along three different crystal directions: along $\langle 001\rangle$ and within the *ab* plane along $\langle 100\rangle$ and $\langle 110\rangle$ directions. The susceptibility in each case is on the order of $10^{-4}$ matching the calculated value of $3.98\times10^{-4}$ for $Mn_2Au$ in the literature [8]. The hysteresis at room temperature and the steep slopes at low temperature are attributed to the trace MnBi impurity still remaining on the samples. The hierarchy of $\chi_{110}$ being larger than $\chi_{100}$ is repeated in the acid-cleaned sample in Fig. S7 too, whereas exact magnitudes of susceptibility vary due to the varying degree of contribution of the FM component in different samples.

The susceptibility measured with field along the $\langle 110\rangle$ crystal direction is the largest at both temperatures. Susceptibility along $\langle 110\rangle$, $\chi_{110}$, is 1.42 and 1.6 times larger than that along $\langle 100\rangle$, $\chi_{100}$, at 10 K and 300 K respectively. Whereas $\chi_{110}$ is only 1.05 times larger than susceptibility along $\langle 001\rangle$, $\chi_{001}$, at 10 K. At room temperature the difference widens with $\chi_{110}$ 1.25 times larger than $\chi_{001}$. This hierarchy is reproducible in different samples.

## 3 Measuring In-plane Anisotropic Susceptibility

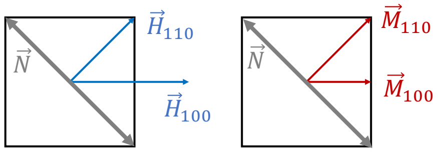


First let us assume that no large magnetic reorientation is occurring due to applied field and $Mn_2Au$ has a preferred Néel direction $N$ that creates two domains $\langle 110\rangle$ and $\langle 1\bar{1}0\rangle$. Susceptibility will be maximized when measuring normal to a Néel vector due to spin canting. Measuring the susceptibility $\chi_{100}$ (45° from the Néel vector) can be treated as the sample having one full domain with $\langle 110\rangle$ Néel vector (both domains have equivalent response). The applied field projected on the domain is

$$H_{110} = \frac{H_{100}}{\sqrt{2}} \tag{1}$$

So the moment projected back into the measurement direction is

$$M_{100} = \frac{M_{110}}{\sqrt{2}} \tag{2}$$

Measured susceptibility is experimentally obtained as the ratio of $M$ to $H$:

$$\chi_{100} = \frac{M_{100}}{H_{100}} \tag{3}$$

Substituting Eq. 2 gives:

$$\chi_{100} = \frac{M_{110}}{\sqrt{2}} \cdot \frac{1}{H_{100}} \tag{4}$$

And substituting the definition $M_{110} = \chi_{110} H_{110}$:

$$\chi_{100} = \frac{\chi_{110} H_{110}}{\sqrt{2}} \cdot \frac{1}{H_{100}} \tag{5}$$

Projecting $H_{110}$ from Eq. 1 gives:

$$\chi_{100} = \frac{\chi_{110} H_{100}}{2} \cdot \frac{1}{H_{100}} = \frac{\chi_{110}}{2} \tag{6}$$

The same construction can be performed for the case where the preferred Néel vector is along $\langle 100\rangle$ and $\chi_{110}$ is measured at 45°. If the susceptibility is instead measured *along* the Néel vector direction then assume half the sample has nonzero $\chi_\perp$ while the rest has $\chi_\parallel = 0$. The susceptibility would then be the same as Eq. 6, i.e. that material has no in-plane magnetic anisotropy.

At higher fields, not accessible in this study, domains with Néel vectors normal to the field direction should grow, while a material with domains 45° to the field direction has no driving force for domain growth (only spin canting) until the field required for a spin flop transition is reached. The lack of steps in our $M/H$ data for $Mn_2Au$ rules out a spin flop transition, and higher fields are necessary to observe this anisotropic behavior.

Table S1: Table of synthesis conditions and the resulting crystal dimensions from variations of flux reactions that yielded $Mn_2Au$ crystals. Mn, Au, and Bi are the nominal molar ratios of precursors. Key processing temperature profile features are listed. $T_{hold}$ is the maximum temperature at which the mixture was held for $t_i$ (hr) amount of time. A hold time $t_{650-665°C}$ at intermediate temperatures of 650 to 665°C and the total cooling time below this intermediate temperature before quenching at 470°C are both varied across different recipe variations. The largest exposed area of the largest sample in each batch is logged as $A$, and the estimated volume of the crystal assuming the thickness and cross-sectional width are equal is logged as $V$.

| **Name** | **Mn** | **Au** | **Bi** | $t_i$**(hr)** | $T_{hold}$ **(°C)** | $A$ **(mm$^2$)** | $V$ **(mm$^3$)** | $t_{650-665°C}$ **(hr)** | $t_{T<650-665°C}$ **(hr)** |
|---|---|---|---|---|---|---|---|---|---|
| **MSG1004** | 3.3 | 1 | 12 | 12 | 750 | 0.39 | 0.09 | 24 | 48 |
| **MSG1009** | 3.3 | 1 | 12 | 12 | 750 | 0.36 | 0.06 | 72 | 180 |
| **MSG1010** | 3.3 | 1 | 12 | 12 | 750 | 0.26 | 0.08 | 24 | 85 |
| **MSG1012** | 3.3 | 1 | 12 | 12 | 750 | 0.21 | 0.02 | 48 | 114 |
| **RB1001** | 2 | 1 | 4 | 12 | 700 | 0.11 | 0.01 | 0 | 18 |
| **RB1003** | 2 | 1 | 4 | 12 | 700 | 0.16 | 0.02 | 0 | 13 |
| **RB1004** | 5 | 1 | 12 | 12 | 750 | 0.35 | 0.07 | 0 | 64 |
| **RB1005** | 5 | 1 | 12 | 12 | 750 | 0.65 | 0.10 | 24 | 72 |
| **RB1010** | 5 | 1 | 12 | 12 | 750 | 0.34 | 0.05 | 24 | 72 |
| **RB1012** | 7 | 1 | 12 | 12 | 750 | 2.52 | 0.25 | 24 | 72 |
| **RB1013** | 5 | 1 | 12 | 12 | 750 | 0.16 | 0.02 | 24 | 72 |
| **RB1015** | 4 | 1 | 8 | 12 | 750 | 0.20 | 0.05 | 24 | 72 |
| **RB1019** | 5 | 1 | 12 | 12 | 750 | 0.46 | 0.12 | 24 | 72 |
| **Rb1020** | 7 | 1 | 12 | 12 | 750 | 1.21 | 0.12 | 24 | 72 |
| **RB1021** | 5 | 1 | 12 | 12 | 750 | 0.38 | 0.06 | 48 | 96 |
| **RB1024** | 5 | 1 | 12 | 12 | 750 | 0.53 | 0.05 | 24 | 72 |
| **RB1025** | 7 | 1 | 12 | 12 | 750 | 0.15 | 0.03 | 24 | 72 |
| **RB1026** | 9 | 1 | 12 | 12 | 750 | 0.63 | 0.06 | 24 | 72 |
| **RB1027** | 7 | 1 | 14 | 12 | 750 | 1.04 | 0.30 | 24 | 72 |
| **RB1029** | 5 | 1 | 12 | 12 | 750 | 0.32 | 0.06 | 24 | 72 |
| **RB1031** | 7 | 1 | 12 | 12 | 750 | 0.28 | 0.03 | 24 | 76 |
| **RB1032** | 7 | 1 | 12 | 12 | 700 | 1.04 | 0.10 | 0 | 100 |
| **RB1033** | 7 | 1 | 12 | 48 | 550 | 0.15 | 0.03 | 0 | 69 |
| **RB1035** | 7 | 1 | 16 | 12 | 750 | 0.40 | 0.06 | 24 | 72 |
| **RB1036** | 7 | 1 | 20 | 12 | 750 | 0.75 | 0.16 | 24 | 72 |
| **RB1037** | 7 | 1 | 12 | 12 | 750 | 0.38 | 0.10 | 24 | 120 |
| **RB1038** | 7 | 1 | 12 | 12 | 750 | 0.45 | 0.05 | 24 | 72 |
| **RB1040** | 7 | 1 | 12 | 12 | 750 | 0.62 | 0.18 | 24 | 124 |
| **RB1045** | 7 | 1 | 24 | 12 | 750 | 1.11 | 0.30 | 24 | 72 |
| **RB1046** | 9 | 1 | 20 | 12 | 750 | 3.02 | 1.07 | 24 | 72 |

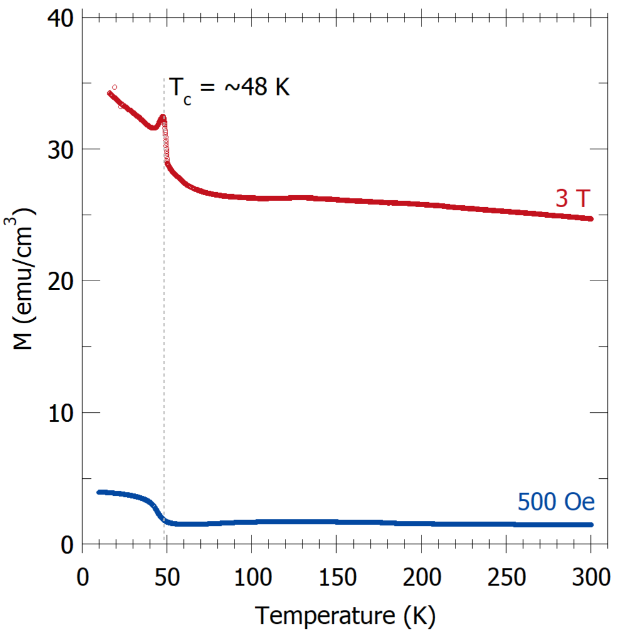


Figure S2: Magnetization versus temperature plot of a $Mn_2Au$ sample that was previously heated to 700 K in helium atmosphere to measure magnetic susceptibility. A feature at $\sim$48 K indicates the ferrimagnetic Curie temperature of $Mn_3O_4$. [9] This shows that a small $Mn_3O_4$ forms on the surface of the sample when heated in the Magnetic Property Measurement System for high temperature characterization. Prior to both measurements, the sample was gently scraped to remove loosely-attached flux. This is the same sample as shown in Figures S4 and S5.

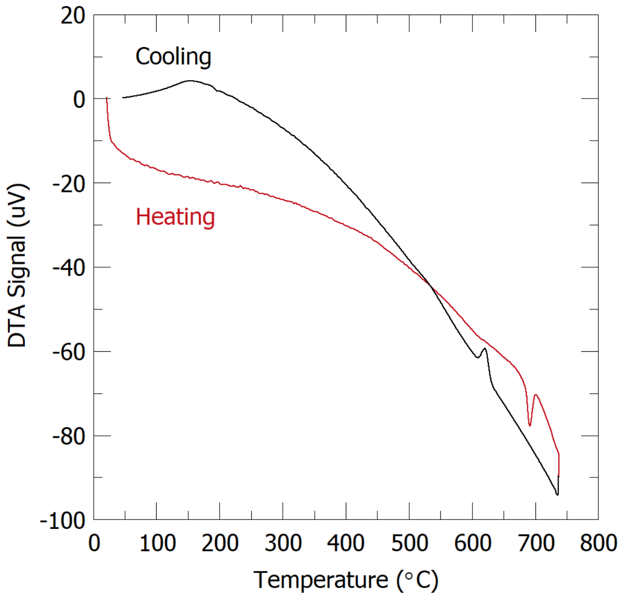


Figure S3: Differential thermal analysis (DTA) on pure $Mn_2Au$ between room temperature and 750° C shows a decomposition on heating, with an onset around 680°C, which is the incongruent decomposition of $Mn_2Au$ to an ordered MnAu phase and fcc solid solution that extends to the elemental allotrope $\gamma$-Mn, in agreement with the published Mn–Au phase diagram.[10], The onset of the feature upon cooling is about 640°C.

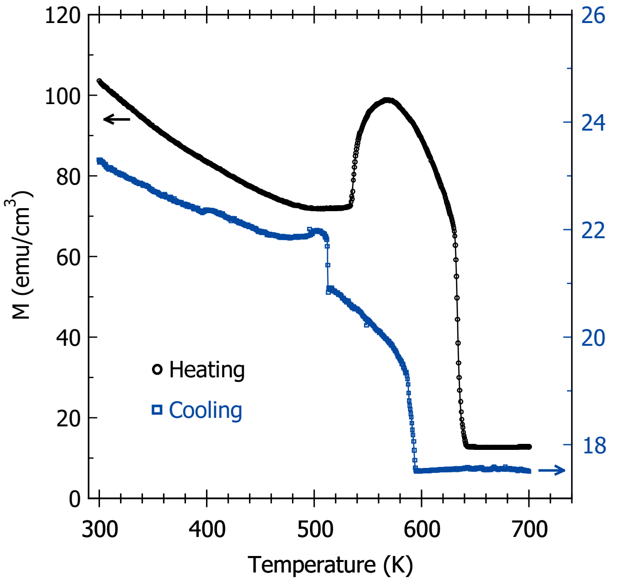


Figure S4: Magnetic moment versus temperature of $Mn_2Au$ with a ferromagnetic impurity shows that upon heating (black), the moment drops at around 630 K, which is the temperature where the low-temperature phase (LTP) of MnBi decomposes into the paramagnetic phases $Mn_{1.08}Bi$ and Bi.[1] The magnitude of magnetic moment and ordering transition temperature are irreversible upon slow cooling, and the different $y$-axis scales indicate a partial suppression of the formation of ferromagnetic LTP-MnBi.

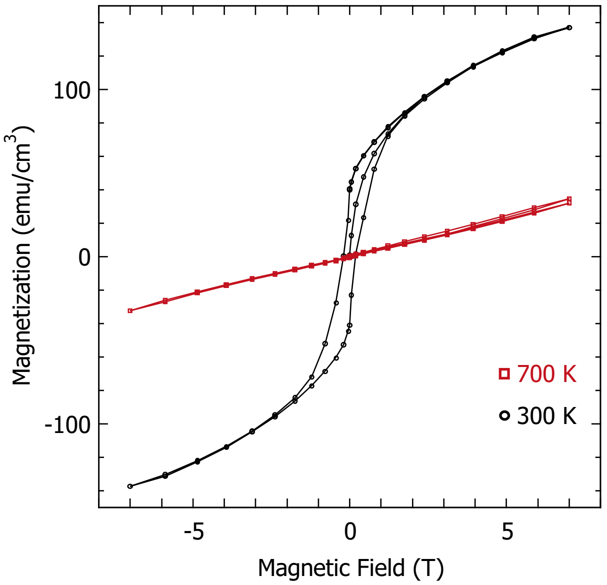


Figure S5: Magnetic moment versus applied field for a $Mn_2Au$ sample at room temperature and at 700 K, above the Curie temperature of MnBi impurity. The hysteresis and large magnitude of $M$ at 300 K disappear in the paramagnetic regime of MnBi at 700 K.

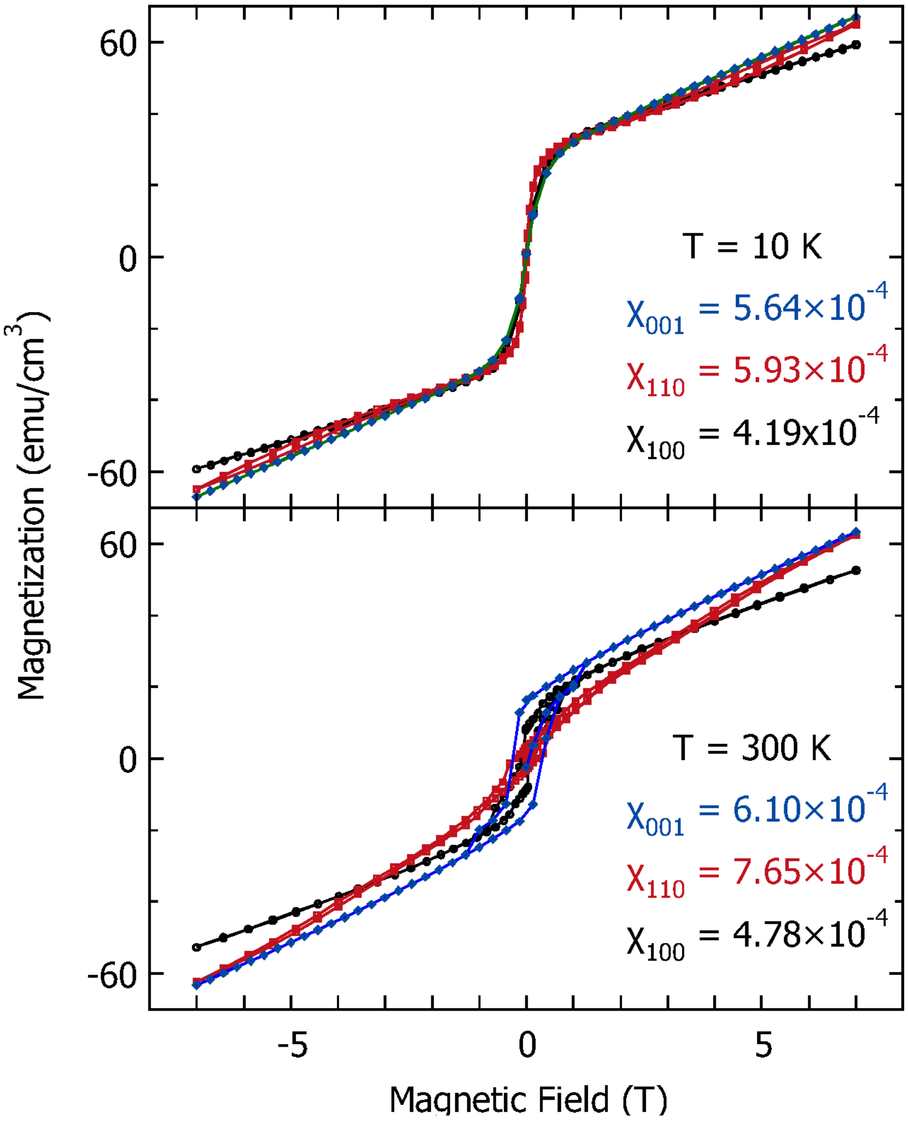


Figure S6: Magnetization versus field isotherms at 10 K and 300 K with field applied along the $\langle 001 \rangle, \langle 110 \rangle$, and $\langle 100 \rangle$ crystal directions show evidence of out-of-plane and in-plane anisotropy. This sample was heated post-synthesis to 700 K and quenched across the MnBi Curie temperature in vacuum to suppress the FM contribution. However, the 700 K heating leads to a FM contribution from $Mn_3O_4$, as shown in Figure S3. Susceptibilities shown are for the high-field regions. Note that all three orientations give similar susceptibilities.

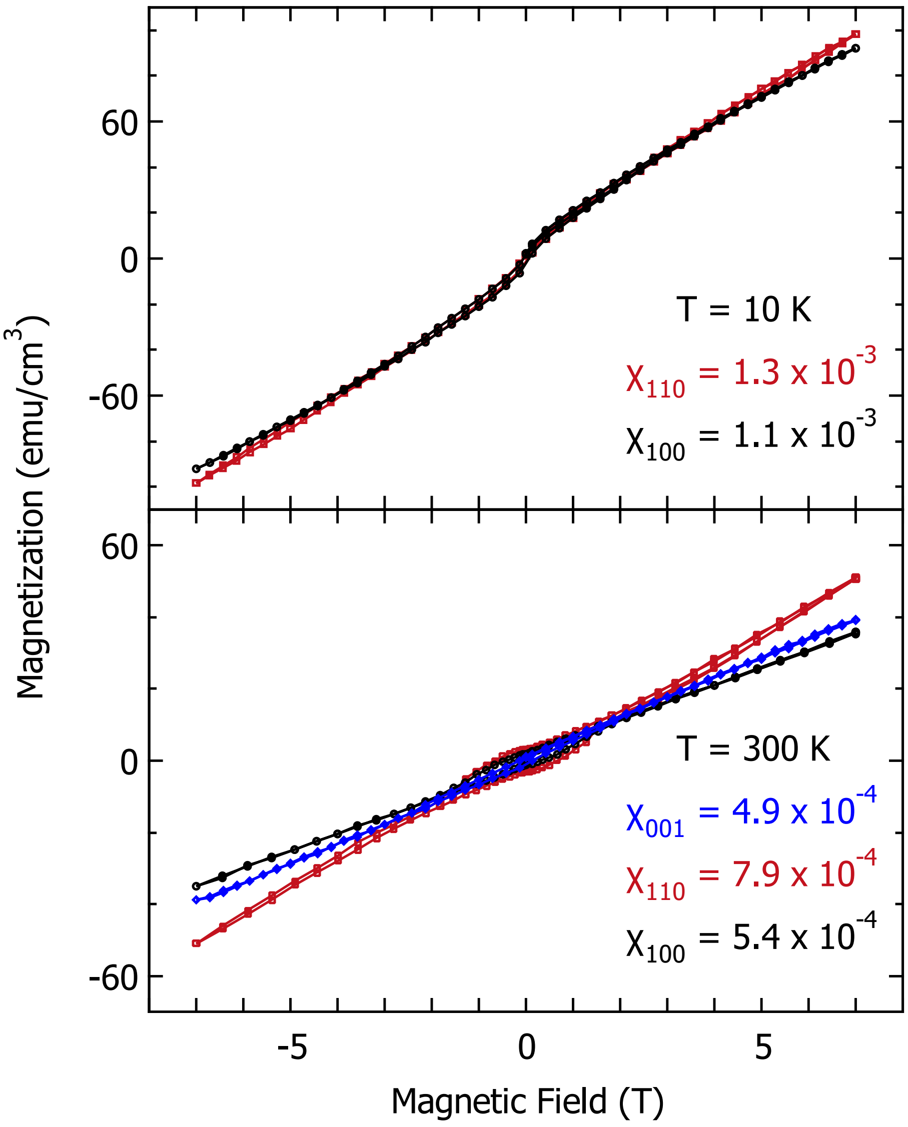


Figure S7: Magnetization versus field isotherms at 10 K and 300 K with field applied along the $\langle 001\rangle, \langle 110\rangle$, and $\langle 100\rangle$ crystal directions. The hierarchy of susceptibilities along $\langle 110\rangle$ and $\langle 100\rangle$ directions is repeatable. This sample was acid-etched to remove remnant surface flux and the FM MnBi impurity, resulting in a much smaller low-field FM contribution than Figure S6, but again $\chi_{001}$ is not significantly different from $\chi_{100}$ or $\chi_{110}$, which should be equivalent by symmetry.

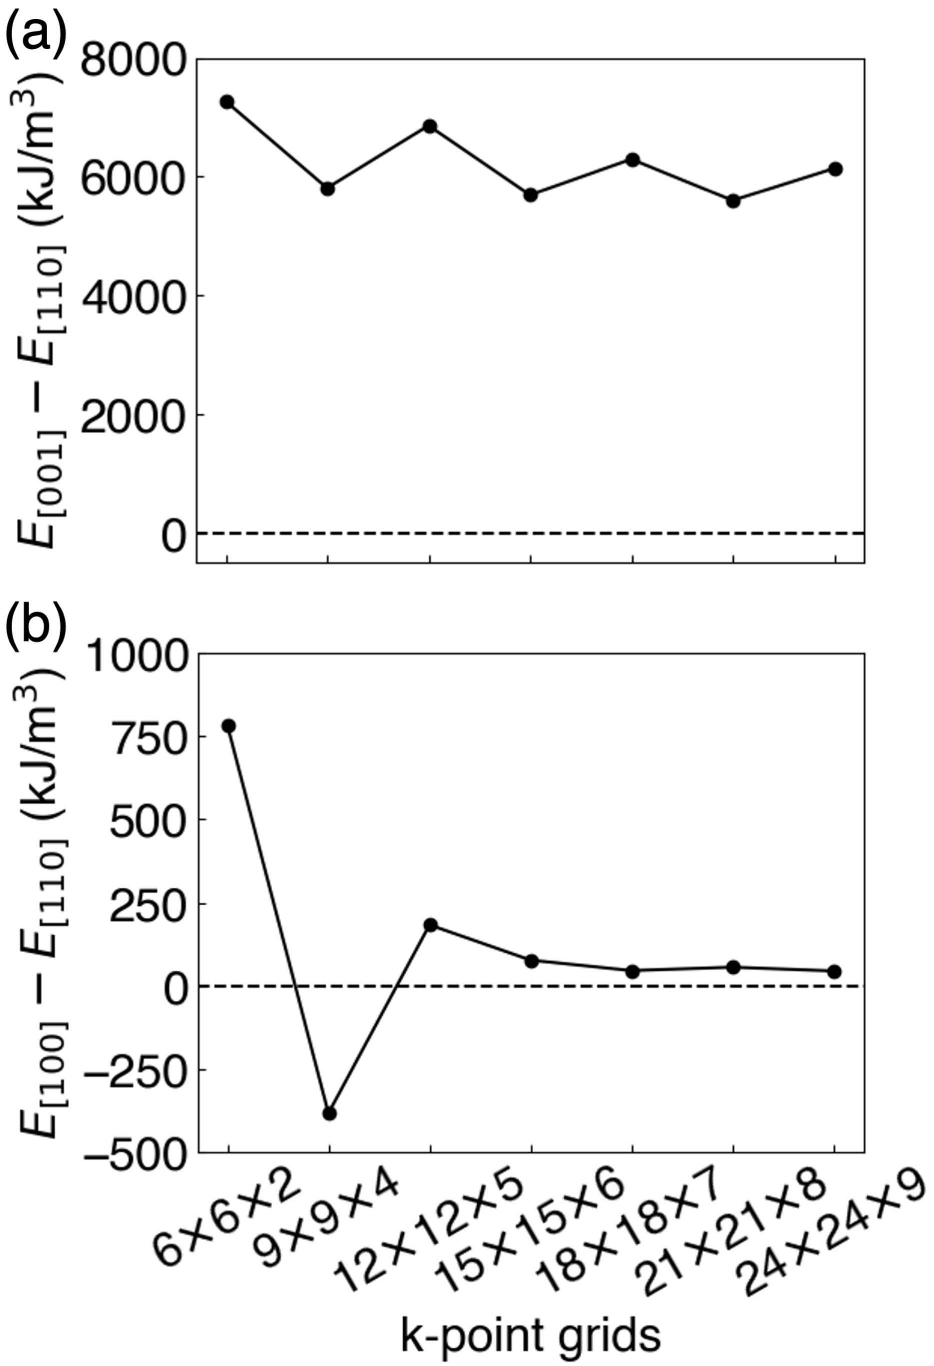


Figure S8: Convergence test for the calculated (a) in-plane and (b) out-of-plane magnetocrystalline anisotropy energy contributed from spin-orbit interaction, as a function of the $k$-point grid.

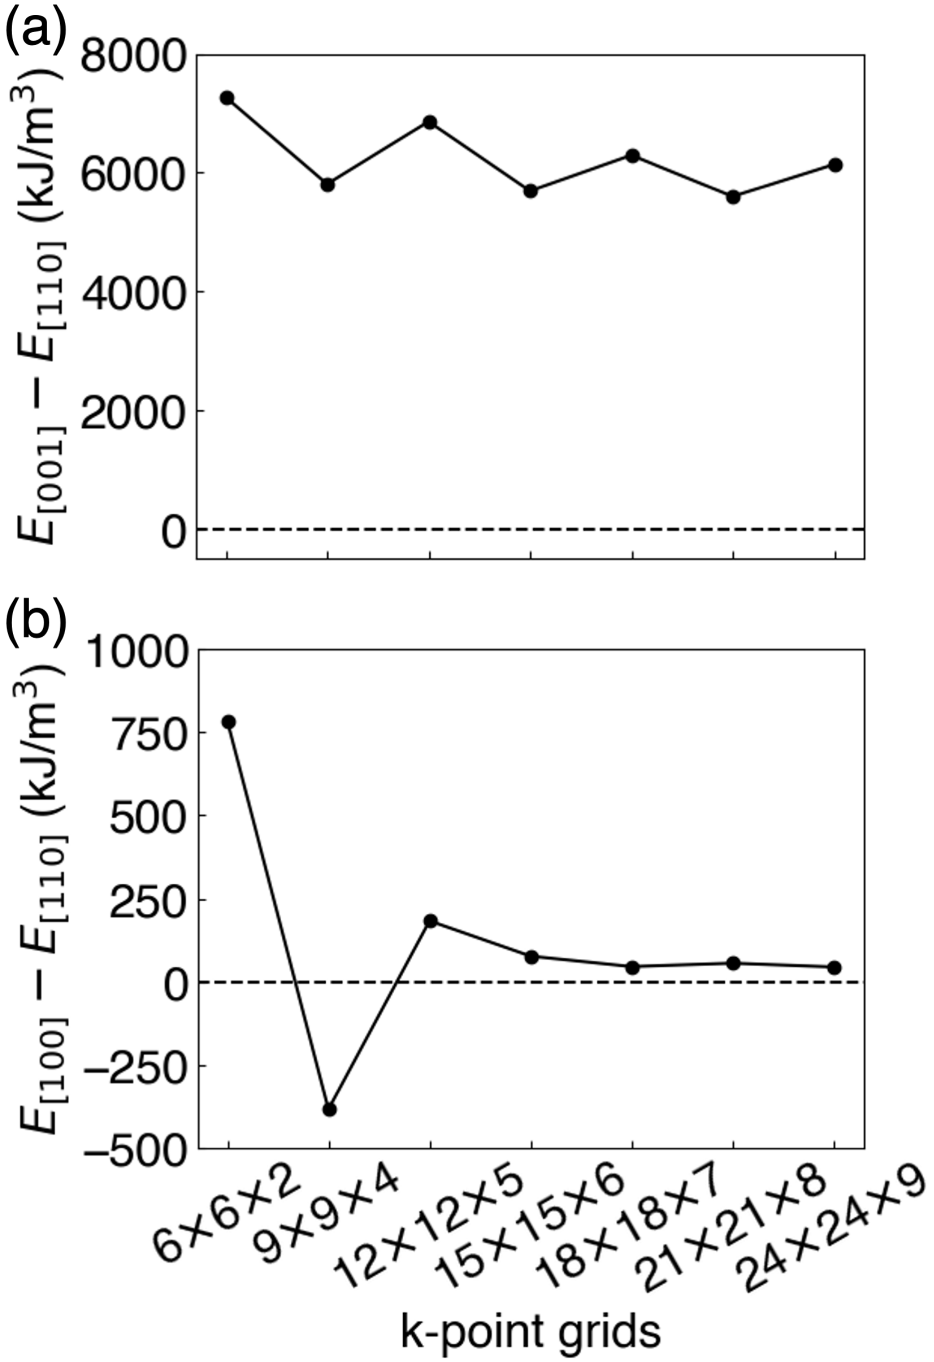


Figure S9: Convergence test for the calculated (a) in-plane and (b) out-of-plane magnetocrystalline anisotropy energy contributed from spin-orbit interaction, as a function of the $k$-point grid.

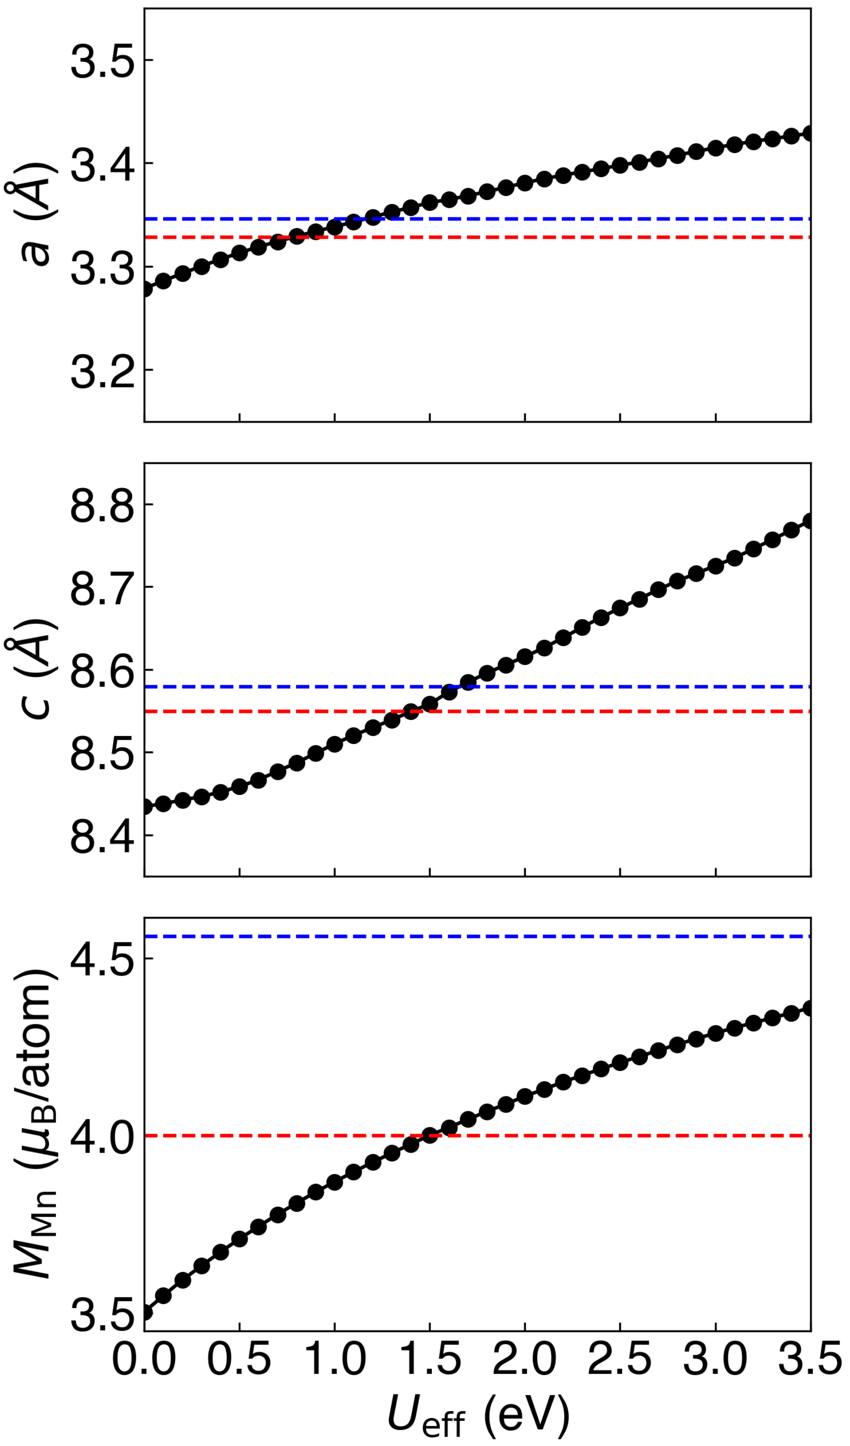


Figure S10: Calculated lattice parameters $a$ and $c$, as well as the magnetic moment on Mn atom ($M_{\mathrm{Mn}}$), of $Mn_2Au$ (black circle markers) as functions of the effective on-site Coulomb interaction parameter ($U_{\mathrm{eff}}$). The blue dashed lines represent measured values obtained from this work. The red dashed lines for lattice parameters and magnetic moments depict values measured in references [34] and [18] in the main text.

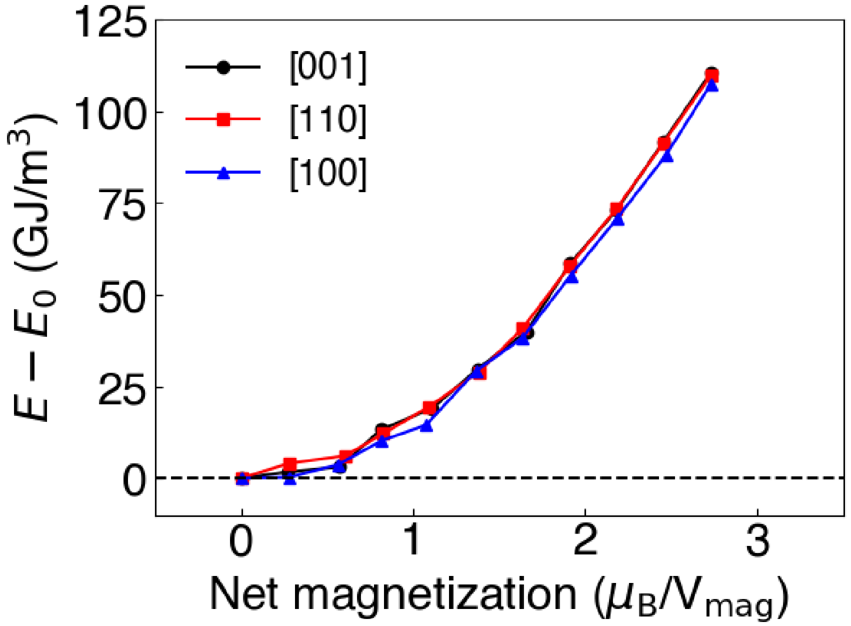


Figure S11: Calculated total energy curves for $Mn_2Au$ with the magnetic moment tilted along ⟨100⟩, ⟨110⟩, and ⟨001⟩ directions, plotted as a function of the net magnetization per magnetic unit cell volume ($V_{mag}$). The total energy change is expressed in gigajoules per cubic meter.

# References


[1] M. A. McGuire, H. Cao, B. C. Chakoumakos, and B. C. Sales. Symmetry-lowering lattice distortion at the spin reorientation in MnBi single crystals. *Phys. Rev. B*, 90(17):174425, 2014.

[2] V. M. T. S. Barthem, C. V. Colin, H. Mayaffre, M.-H. Julien, and D. Givord. Revealing the properties of $Mn_2Au$ for antiferromagnetic spintronics. *Nat. Commun.*, 4(1):2892, 2013.

[3] J. Cui, J. P. Choi, G. Li, E. Polikarpov, J. Darsell, N. Overman, M. Olszta, D. Schreiber, M. Bowden, T. Droubay, M. J. Kramer, N. A. Zarkevich, L. L. Wang, D. D. Johnson, M. Marinescu, I. Takeuchi, Q. Z. Huang, H. Wu, H. Reeve, N. V. Vuong, and J. P. Liu. Thermal stability of MnBi magnetic materials. *J. Phys.: Condens. Matter*, 26(6):064212, 2014.

[4] A. F. Andresen, W. Hälg, P. Fischer, E. Stoll, G. Eriksson, R. Blinc, S. Paušak, L. Ehrenberg, and J. Dumanović. The magnetic and crystallographic properties of MnBi studied by neutron diffraction. *Acta Chem. Scand.*, 21:1543–1554, 1967.

[5] V. Taufour, S. Thimmaiah, S. March, S. Saunders, K. Sun, T. N. Lamichhane, M. J. Kramer, S. L. Bud'ko, and P. C. Canfield. Structural and ferromagnetic properties of an orthorhombic phase of MnBi stabilized with Rh additions. *Phys. Rev. Applied*, 4(1):014021, 2015.

[6] M. N. El Hazek and A. A. Gabr. Dissolution of Manganese from Polymetallic Material Using Sulfuric-Oxalic Acid Medium. *Am. J. Analyt. Chem.*, 7(5):469–477, May 2016.

[7] V. Lenher. Solubility of gold in certain oxidizing agents. *J. Am. Chem. Soc.*, 26(5):550–554, 1904.

[8] K. Kang, K. Yang, K. Puthalath, D. G. Cahill, and A. Schleife. Polar magneto-optical Kerr effect in antiferromagnetic $M_2As$ ($M$ = Cr, Mn, Fe) under an external magnetic field. *Phys. Rev. B*, 105(18):184404, 2022.

[9] Lakshmi Narayani, V. Jagadeesha Angadi, Anu Sukhdev, Malathi Challa, Shidaling Matteppanavar, P. R. Deepthi, P. Mohan Kumar, and Mehaboob Pasha. Mechanism of high temperature induced phase transformation and magnetic properties of $Mn_3O_4$ crystallites. *J. Magn. Magn. Mater.*, 476:268–273, 2019.

[10] P. Wells and J. H. Smith. The structure of $Mn_2Au$ and $Mn_3Au$. *Acta Crystallographica Section A*, 26(3):379–381, May 1970.
